# Supplementary material for: On the Approximability of Related Machine Scheduling under Arbitrary Precedence
Source: arXiv:1711.09964 source file (2021-04-07)
Supplement: Supplementary file 1 [file 7_appendix.tex]

\section{Appendix}
